# Supplementary material for: hyppo: A Multivariate Hypothesis Testing Python Package
Source: arXiv:1907.02088 source file (2024-09-13)
Supplement: Supplementary file 1 [file appendix.tex]

\appendix

%===============================================================================%
% Statistics
%===============================================================================%
\section{Mathematical Details}
\label{app_math}

This section overviews comparisons between the independence tests that were implemented in this package. Information pertaining to the other modules can be found
for time-series independence testing in \citet{mehta2019consistent} and
for \ksample~testing
and random-forest based independence and \ksample~testing in an upcoming manuscript.

All independence tests can be generalized into the following form: given random variables $X$ and $Y$, which are assumed to be from the joint distribution $F_{XY} = F_{X | Y} F_Y$, two variables are considered independent if and only if $F_{X | Y} F_Y = F_X F_Y$; that is, the joint distribution is equal to the product of the marginals. This idea can be formulated as the following test:
\[
    \begin{split}
        H_0 : F_{XY} &= F_X F_Y, \\
        H_A : F_{XY} &\neq F_X F_Y.
    \end{split}
\]
It turns out any dependency measure can be directly used to test equality of two or more distributions, i.e., two-sample or K-sample test, see \cite{shen2018exact}.

\subsection{Notation}
Let $\Real$ denote the real line $\left( -\infty, \infty \right)$. Let $F_X$, $F_Y$, and $F_{XY}$ refer to the marginal and joint distributions of random variables $X$ and $Y$ respectively. Let $x$ and $y$ refer to the samples from $F_X$ and $F_Y$ and $\ve{x} \in \Real^{n \times p} $ and $\ve{y} \in \Real^{n \times q}$ refer to the matrix of these observations. That is, $\ve{x} = \{ x_i \sim F_{X}\ \textrm{where}\ x_i \in \Real^p,\ i = 1,...,n \}$ and $\ve{y} = \{ y_i \sim F_{Y}\ \textrm{where}\ y_i \in \Real^q,\ i = 1,...,n \}$. The trace of an $n \times n$ square matrix is the sum of the elements along the main diagonal; that is, the trace of $n \times n$ matrix $\ve{x}$ is $\trace{\ve{x}} = \sum_{i=1}^n x_{ii}$.

\subsection[Pearson's Product-Moment Correlation Coefficient (Pearson), RV, and Canonical-Correlation Analysis (CCA)]{Pearson's Product-Moment Correlation Coefficient (\Pearson), \RV, and Canonical-Correlation Analysis (\CCA)}

\Pearson~is a measure of the linear correlation between two univariate random variables \citep{pearson1895vii}.
Given sample data $\ve{x}$ and $\ve{y}$ where $p = q = 1$, the sample Pearson correlation is
\begin{equation} \label{eq:genpearson}
    \text{\Pearson}_n \left( \ve{x}, \ve{y} \right) = \frac{\hat{\cov} \left( \ve{x}, \ve{y} \right)}{\hat{\sigma}_{\ve{x}} \hat{\sigma}_{\ve{y}}},
\end{equation}
where $\hat{\cov} \left( \ve{x}, \ve{y} \right)$ is the sample covariance, $\hat{\sigma}_{\ve{x}}$ and $\hat{\sigma}_{\ve{y}}$ are the sample standard deviations of $\ve{x}$ and $\ve{y}$ respectively.

\RV~is a multivariate generalization of the squared \Pearson~coefficient \citep{escoufier1973traitement, robert1976unifying}. The derivation is as follows: assuming each column in $\ve{x}$ and $\ve{y}$ are pre-centered to zero mean in each dimension, then the sample covariance matrix is $\ve{\hat{\Sigma}_{xy}} =  {\ve{x}} \TT \ve{y} $, and the \RV~coefficient is
\begin{equation} \label{eq:rv}
    \text{\RV}_n \left( \ve{x}, \ve{y} \right) = \frac{\trace{\ve{\hat{\Sigma}_{xy}} \ve{\hat{\Sigma}_{yx}}} }{\trace{\ve{\hat{\Sigma}^2_{xx}}} \trace{\ve{\hat{\Sigma}^2_{yy}} }}.
\end{equation}
Another similarly defined tool is \CCA, which  finds the linear combinations with respect to the dimensions of $\ve{x}$ and $\ve{y}$ that maximize their correlation \citep{hardoon2004canonical}. 
It seeks a vector $\ve{a} \in {\Real}^p$ and $\ve{b} \in {\Real}^q$ to compute the first correlation coefficient as
\begin{equation} \label{eq:tomaxcca}
 \max_{\ve{a} \in {\Real}^n, \ve{b} \in {\Real}^m}{ \frac{{\ve{a}} \TT \ve{\hat{\Sigma}_{xy} b}}{\sqrt{{\ve{a}} \TT \ve{\hat{\Sigma}_{xx} a}} \sqrt{{\ve{b}} \TT \ve{\hat{\Sigma}_{yy} b}}}}.
\end{equation}
One can keep on deriving the second and the third canonical correlation coefficients in a similar manner until the end, and \CCA~can also be generalized to more than two random variables (\citep{ShenSunTangPriebe2014}). Therefore, \CCA~can be used to define a test statistic for dependence, and usually people take the first correlation coefficient or the sum of all correlation coefficients as the statistic.
\subsection[Kendall and Spearman]{Kendall (\Kendall) and Spearman (\Spearman)}
\Kendall~and \Spearman~are  rank-based correlation coefficients that are robust univariate test statistics \citep{kendall1938new, spearman1904proof}.
To formulate \Kendall, define $\left( x_i, y_i \right)$ and $\left( x_j, y_j \right)$ as concordant if the ranks agree: $x_i > x_j$ and $y_i > y_j$ or $x_i < x_j$ and $y_i < y_j$. They are discordant if the ranks disagree: $x_i > x_j$ and $y_i < y_j$ or $x_i < x_j$ and $y_i > y_j$. If $x_i = x_j$ and $y_i = y_j$, the pair is said to be tied. Let $n_c$ and $n_d$ be the number of concordant and discordant pairs respectively and $n_0 = n \left( n - 1 \right) / 2$. In the case of no ties, the test statistic is defined as
\begin{equation} \label{eq:tauA}
    \text{\Kendall}_n = \frac{n_c - n_d}{n_0},
\end{equation}
Further define 
\begin{align*}
    n_1 &= \sum_i \frac{t_i \left( t_i - 1 \right)}{2}, \\
    n_2 &= \sum_j \frac{u_j \left( u_j - 1 \right)}{2}, \\
    t_i &= \mathrm{number\ of\ tied\ values\ in\ the}\ i \mathrm{th\ group\ of\ ties\ in\ the\ first\ quantity\, and},  \\
    u_j &= \mathrm{number\ of\ tied\ values\ in\ the}\ j \mathrm{th\ group\ of\ ties\ in\ the\ second\ quantity}.
\end{align*}
In the case of ties, the statistic is calculated as in \cite{agresti2010analysis}
\begin{equation} \label{eq:tauB}
    \text{\Kendall}_n = \frac{n_c - n_d}{\sqrt{\left( n_0 - n_1 \right) \left( n_0 - n_2 \right)}},
\end{equation}
\Spearman~can be thought of as closely related to \Pearson, whose statistic is listed in Equation \ref{eq:genpearson}. Suppose that $\mathrm{rg}_{x_i}$ and $\mathrm{rg}_{y_i}$ are the respective ranks of $n$ raw scores $x_i$ and $y_i$, $\rho$ denotes the \Pearson~coefficient but applied to rank variables, $\cov \left( \mathrm{rg}_{\ve{x}}, \mathrm{rg}_{\ve{y}} \right)$ denotes the covariance of the rank variables, and $\hat{\sigma}_{\mathrm{rg}_{\ve{x}}}$ and  $\hat{\sigma}_{\mathrm{rg}_{\ve{y}}}$ denote the standard deviations of the rank variables. The statistic is
\begin{equation} \label{eq:spearman}
    \text{\Spearman}_s = \rho_{\mathrm{rg}_{\ve{x}}, \mathrm{rg}_{\ve{y}}} = \frac{\cov \left( \mathrm{rg}_{\ve{x}}, \mathrm{rg}_{\ve{y}} \right)}{\hat{\sigma}_{\mathrm{rg}_{\ve{x}}} \hat{\sigma}_{\mathrm{rg}_{\ve{y}}}}.
\end{equation}

\subsection[Mantel]{\Mantel}
\Mantel~is one of the earliest distance-based statistic for independence \citep{mantel1967detection}, which achieves some success in testing without consistency testing (\Mantel~is later shown to be not consistent, see \cite{lyons2013distance, mgc2}). Given $\ve{x}$ and $\ve{y}$, suppose that an appropriate distance measure is used to calculate two  $n \times n$ distance matrices ${\ve{D}}^{\ve{x}}$ and ${\ve{D}}^{\ve{y}}$ respectively, e.g., Euclidean distance. Let the centered matrix be calculated as,
\[
{\ve{C}_{ij}}^{\ve{x}} = {\ve{D}_{ij}}^{\ve{x}} - \frac{1}{n (n - 1)} \sum_{i, j = 1}^n {\ve{D}_{ij}}^{\ve{x}},
\]
similarly for ${\ve{C}}^{\ve{y}}$. Consider a function of $\ve{x}$ and $\ve{y}$, $M$, such that,
\[
M_n \left( \ve{x}, \ve{y} \right) = \trace{{\ve{C}}^{\ve{x}} {\ve{C}}^{\ve{y}}}.
\]
Then, the \Mantel~coefficient is calculated as,
\begin{equation}
    \text{\Mantel}_n \left( \ve{x}, \ve{y} \right) = \frac{M_n \left( \ve{x}, \ve{y} \right)}{\sqrt{M_n \left( \ve{x}, \ve{x} \right) M_n \left( \ve{y}, \ve{y} \right)}}.
\end{equation}
%
%@sampan: I put Mantel before HHG & MDMR. Also, the mantel described here was not correct, I removed it for now & please see my mgc jasa paper for it.

\subsection[Heller, Heller, and Gorfine's (HHG)]{Heller, Heller, and Gorfine's (\Hhg)}
\begin{table}[!tbh]
\centering
\begin{tabular}{|c|c|c|c|}
 \hline
 & $d_{\ve{y}} \left( y_i, \cdot \right) \leq d_{\ve{y}} \left( y_i, y_j \right)$ & $d_{\ve{y}} \left( y_i, \cdot \right) > d_{\ve{y}} \left( y_i, y_j \right)$ & \\
 \hline
 $d_{\ve{x}} \left( x_i, \cdot \right) \leq d_{\ve{x}} \left( x_i, x_j \right)$ & $A_{11} \left(i, j \right)$ & $A_{12} \left(i, j \right)$ & $A_{1 \cdot} \left(i, j \right)$ \\
 \hline
 $d_{\ve{x}} \left( x_i, \cdot \right) > d_{\ve{x}} \left( x_i, x_j \right)$ & $A_{21} \left(i, j \right)$ & $A_{22} \left(i, j \right)$ & $A_{2 \cdot} \left(i, j \right)$ \\
 \hline
  & $A_{\cdot 1} \left(i, j \right)$ & $A_{\cdot 2} \left(i, j \right)$ & $n - 2$ \\
 \hline
\end{tabular}
\caption{The cross-cross classification table used to calculate the Pearson's chi squared test statistic involved in the \Hhg~test statistic calculation.}
\label{tab:crossclassradii}
\end{table}
\Hhg~is a consistent multivariate test of associations based on the rank of the distances \citep{heller2012consistent}. For every sample point $j \neq i$, denote a point in the joint sample space as $\left( x_j, y_j \right)$. Let $d_{\ve{x}} \left( x_i, x_j \right)$ be equivalent to the norm distance between samples $x_i$ and $x_j$ and $d_{\ve{y}} \left( y_i, y_j \right)$ is similarly defined. The indicator function is denoted by $\II \{ \cdot \}$. The cross-classification between these two random variables can be formulated as in Table \ref{tab:crossclassradii}, where

\[
    A_{11} = \sum_{k = 1, k \neq i, j}^n \II \left\{ d_{\ve{x}} \left( x_i, x_k \right) \leq d_{\ve{x}} \left( x_i, x_j \right) \right\} \II \left\{ d_{\ve{y}} \left( y_i, y_k \right) \leq d_{\ve{y}} \left( y_i, y_j \right) \right\},
\]
\noindent and $A_{12}$, $A_{21}$, and $A_{22}$ are defined similarly. $A_{\cdot 1}$, $A_{\cdot 2}$, $A_{1 \cdot}$, and $A_{2 \cdot}$ are the sums of the column and row respectively.
Once this table is generated, the Pearson's chi square test statistic can be calculated using
\[
    S \left( i, j \right) = \frac{\left( n - 2 \right) {\left( A_{12} A_{21} - A_{11} A_{22} \right)}^2}{A_{1 \cdot} A_{2 \cdot} A_{\cdot 1} A_{\cdot 2}}.
\]
From here, the \Hhg~test statistic is simply
\begin{equation} \label{eq:hhg}
    \text{\Hhg}_n = \sum_{i = 1}^n \sum_{j = 1, j \neq i}^n S \left( i, j \right).
\end{equation}

\subsection[Hilbert-Schmidt Criterion (Hsic)]{Hilbert-Schmidt Criterion (\Hsic)}
\Hsic~is a way to measure multivariate nonlinear associations given a specified kernel \citep{gretton2008kernel}. Let ${\ve{K}}^{\ve{x}}$ be an $n \times n$ kernel matrix of $\ve{x}$ and ${\ve{K}}^{\ve{y}}$ be an $n \times n$ kernel matrix of $\ve{y}$. In addition, $\ve{H} = \ve{I} - \left( 1 / n \right) \ve{J}$ and is an $n \times n$ centering matrix, where $\ve{I}$ is the identify matrix of size $n \times n$ and $\ve{J}$ is a matrix of ones that is the same size. Then, $\Hsic$ is defined as
\begin{equation}
    \text{\Hsic}_n \left( \ve{x}, \ve{y} \right) = \frac{1}{n^2} \trace {{\ve{K}}^{\ve{x}} \ve{H} {\ve{K}}^{\ve{y}} \ve{H}}.
\end{equation}
The default kernel choice is the Gaussian kernel using the median distance as the bandwidth, which is a characteristic kernel that guarantees \Hsic~being a consistent test \citep{gretton2008kernel,gretton2010consistent}. Specifically, the Gaussian kernel transformation for $\ve{x}$  of the form $\mathcal{N} \left( 0, \med{ \left( x_i - x_j \right) } \right)$ where $\med$ refers to the dimension-wise median of $\ve{x}$. The transformation for $\ve{y}$ is defined similarly. We adopt this convention in \mgcpy. 

\subsection[Distance Correlation (Dcorr) and Unbiased Dcorr (UDcorr)]{Distance Correlation (\Dcorr) and Unbiased \Dcorr~(\UDcorr)}
\Dcorr~can be used to measure linear and nonlinear associations between two random vectors of arbitrary dimension. Let ${\ve{D}}^{\ve{x}}$ be the $n \times n$ distance matrix of $\ve{x}$ and ${\ve{D}}^{\ve{y}}$ be the $n \times n$ distance matrix of $\ve{y}$.
The distance covariance (\Dcov) is defined as
\begin{equation} \label{eq:dcovhsic}
    \text{\Dcov}_n \left( \ve{x}, \ve{y} \right) = \frac{1}{n^2} \trace {{\ve{D}}^{\ve{x}} \ve{H} {\ve{D}}^{\ve{y}} \ve{H}}.
\end{equation}
The normalized version of this covariance is $\Dcorr$ \citep{szekely2007measuring} and can be calculated as
\begin{equation}  \label{eq:dcorr}
    \text{\Dcorr}_n \left( \ve{x}, \ve{y} \right) = \frac{\Dcov_n \left( \ve{x}, \ve{y} \right)}{\sqrt{\Dcov_n \left( \ve{x}, \ve{x} \right) \Dcov_n \left( \ve{y}, \ve{y} \right)}}.
\end{equation}
\Dcorr~is almost the same as \Hsic~except one operates on distance while the other operates on kernel. They are indeed equivalent in the sense that every valid kernel has a corresponding valid semimetric to ensure their equivalence, and vice versa \citep{sejdinovic2013equivalence, shen2018exact}.
The original \Dcorr~(and so does \Hsic) is biased. A modified matrix ${\ve{C}}^{\ve{x}}$ based on $\ve{H} {\ve{D}}^{\ve{x}} \ve{H}$ can be calculated as
\[
{\ve{C}_{ij}}^{\ve{x}} =
\begin{cases}
{\ve{D}_{ij}}^{\ve{x}} - \frac{1}{n - 2} \sum_{t = 1}^n {\ve{D}_{it}}^{\ve{x}} - \frac{1}{n - 2} \sum_{s = 1}^n {\ve{D}_{sj}}^{\ve{x}} + \frac{1}{\left( n - 1 \right) \left( n - 2 \right)} \sum_{s,t = 1}^n {\ve{D}_{st}}^{\ve{x}}& i \neq j \\
0 & \mathrm{otherwise}
\end{cases},
\]
similarly for ${\ve{C}}^{\ve{y}}$. Then
the unbiased \Dcov~(\UDcorr) \citep{SzekelyRizzo2014} is thus
\begin{equation}  \label{eq:unbiaseddcov}
    \text{\UDcov}_n \left( \ve{x}, \ve{y} \right) = \frac{1}{n \left( n - 3 \right)} \trace{{\ve{C}}^{\ve{x}} {\ve{C}}^{\ve{y}}}.
\end{equation}
\UDcorr~can consequently be calculated using equation \ref{eq:dcorr}. Similarly, one can compute the unbiased and normalized version of \Hsic~in the same manner.

\subsection[Multiscale Graph Correlation (MGC)]{Multiscale Graph Correlation (\Mgc)}
\Mgc~is a  generalization of \Dcov~that preserves the consistency property while achieving better power in many typical multivariate non-monotonic settings, which also providing some characterization of the latent geometry of the relationship \citep{vogelstein2019discovering}. It is performed utilizing the following steps:
\begin{enumerate}
    \item Two distance matrices ${\ve{D}}^{\ve{x}}$ and ${\ve{D}}^{\ve{y}} $are computed, and modified to be mean zero column-wise. This results in two $n \times n$ distance matrices ${\ve{C}}^{\ve{x}}$ and ${\ve{C}}^{\ve{y}}$ (the centering and unbiased modification is slightly different from the unbiased modification in the previous section, see \cite{mgc2} for more details).
    \item For all values $k$ and $l$ from $1, ..., n$,
    \begin{enumerate}
        \item The $k$-nearest neighbor and $l$-nearest neighbor graphs are calculated for each property. Here, $\ve{G}_k \left( i, j \right)$ indicates the $k$ smallest values of the $i$-th row of ${\ve{D}}^{\ve{x}}$ and $\ve{H}_l \left( i, j \right)$ indicates the $l$ smallest values of the $i$-th row of ${\ve{D}}^{\ve{y}}$.
        \item Let $\circ$ denotes the entry-wise matrix product, then local correlations are summed and normalized using the following statistic:
        \[
        c^{kl} = \frac{\trace{( {\ve{C}}^{\ve{x}} \circ \ve{G}_k) ({\ve{C}}^{\ve{y}} \circ \ve{H}_l)^{T}}}{\sqrt{\trace{ ({\ve{C}}^{\ve{x}} \circ \ve{G}_k) ({\ve{C}}^{\ve{y}} \circ \ve{H}_l)^{T}}\trace{ ({\ve{C}}^{\ve{x}} \circ \ve{G}_k) ({\ve{C}}^{\ve{y}} \circ \ve{H}_l}^{T})}},
        \]
    \end{enumerate}
    \item The \Mgc~test statistic is the smoothed optimal local correlation of $\left\{ c^{kl} \right\}$. Denote the smoothing operation as $R(\cdot)$ (which essentially set all isolated large correlations as $0$ and connected large correlations same as before, see \cite{mgc2}), \Mgc~is
    \begin{equation}
        \text{\Mgc}_n \left( \ve{x}, \ve{y} \right) = \max_{\left( k, l \right)} R(c^{kl} \left( \ve{x}_n, \ve{y}_n \right)).
    \end{equation}
\end{enumerate}

%===============================================================================%
% Statistics
%===============================================================================%
\section{Simulations}
\label{app_sims}
Simulations for Figures \ref{fig_indep_power_sampsize} and \ref{fig_indep_power_dimension} were generated utilizing the following equations.

\begin{enumerate}
\item \texttt{Linear}$\left( X, Y \right) \in \Real^p \times \Real$:
\[X \sim {\mathcal{U} \left( -1, 1 \right)}^p,\]
\[Y = w \T X + \kappa \epsilon.\]

\item \texttt{Exponential}$\left( X, Y \right) \in \Real^p \times \Real$:
\[X \sim {\mathcal{U} \left( 0, 3 \right)}^p,\]
\[Y = \exp \left( w \T X \right) + 10 \kappa \epsilon.\]

\item \texttt{Cubic}$\left( X, Y \right) \in \Real^p \times \Real$:
\[X \sim {\mathcal{U} \left( -1, 1 \right)}^p,\]
\[Y = 128 {\left( w \T X - \frac{1}{3} \right)}^3 + 48 {\left( w \T X - \frac{1}{3} \right)}^2 - 12 \left( w \T X - \frac{1}{3} \right) + 80 \kappa \epsilon.\]

\item \texttt{Joint\ Normal}$\left ( X, Y \right) \in \Real^p \times \Real^p$: Let $\rho = 1/2 p$, $I_p$ be the identity matrix of size $p \times p$, $J_p$ be the matrix of ones of size $p \times p$, and 
$\Sigma =
\begin{bmatrix}
    I_p & \rho J_p \\
    \rho J_p & \left(1 + 0.5 \kappa \right) I_p\\
\end{bmatrix}$.
Then,
\[\left( X, Y \right) \sim \mathcal{N} \left( 0, \Sigma \right).\]

\item \texttt{Step\ Function}$\left( X, Y \right) \in \Real^p \times \Real$:
\[X \sim {\mathcal{U} \left( -1, 1 \right)}^p,\]
\[Y = \II \left( w \T X > 0 \right) + \epsilon,\]
where $\II$ is the indicator function; that is, $\II \left( z \right)$ is unity whenever $z$ is true, and $0$ otherwise.

\item \texttt{Quadratic}$\left( X, Y \right) \in \Real^p \times \Real$:
\[X \sim {\mathcal{U} \left( -1, 1 \right)}^p,\]
\[Y = {\left( w \T X \right)}^2 + 0.5 \kappa \epsilon.\]

\item \texttt{W-Shape}$\left( X, Y \right) \in \Real^p \times \Real$: For $U \sim {\mathcal{U} \left( -1, 1 \right)}^p$,
\[X \sim {\mathcal{U} \left( -1, 1 \right)}^p,\]
\[Y = 4 \left[ {\left( {\left( w \T X \right)}^2 - \frac{1}{2} \right)}^2 + \frac{w \T U}{500} \right] + 0.5 \kappa \epsilon.\]

\item \texttt{Spiral}$\left( X, Y \right) \in \Real^p \times \Real$: For $U \sim \mathcal{U} \left( 0, 5 \right)$, $\epsilon \sim \mathcal{N} \left( 0, 1 \right)$,
\[X_{\left| d \right|} = U \sin \left(\pi U \right) \cos^d \left(\pi U \right)\ \mathrm{for}\ d = 1, ..., p - 1,\]
\[X_{\left| p \right|} = U \cos^p \left(\pi U \right),\]
\[Y = U \sin \left( \pi U \right) + 0.4 p \epsilon.\]

\item \texttt{Uncorrelated\ Bernoulli}$\left( X, Y \right) \in \Real^p \times \Real$: For $U \sim \mathcal{B} \left( 0.5 \right)$, $\epsilon_1 \sim \mathcal{N} \left( 0, I_p \right)$, $\epsilon_2 \sim \mathcal{N} \left( 0, 1 \right)$,
\[X \sim {\mathcal{B} \left( 0.5 \right)}^p + 0.5 \epsilon_1,\]
\[Y = \left( 2 U - 1 \right) w \T X + 0.5 \epsilon_2.\]

\item \texttt{Logarithmic}$\left( X, Y \right) \in \Real^p \times \Real^p$: For $\epsilon \sim \mathcal{N} \left( 0, I_p \right)$,
\[X \sim \mathcal{N} \left( 0, I_p \right),\]
\[Y_{\left| d \right|} = 2 \log_2 \left( \left| X_{\left| d \right|} \right| \right) + 3 \kappa \epsilon_{\left| d \right|}\ \mathrm{for}\ d = 1, ..., p.\]

\item \texttt{Fourth\ Root}$\left( X, Y \right) \in \Real^p \times \Real$:
\[X \sim {\mathcal{U} \left( -1, 1 \right)}^p,\]
\[Y = {\left| w \T X \right|}^{1/4} + \frac{\kappa}{4} \epsilon.\]

\item \texttt{Sine\ Period\ 4$\pi$}$\left( X, Y \right) \in \Real^p \times \Real^p$: For $U \sim \mathcal{U} \left( -1, 1 \right)$, $V \sim {\mathcal{N} \left( 0, 1 \right)}^p$, $\theta = 4 \pi$,
\[X_{\left| d \right|} = U + 0.02 p V_{\left| d \right|}\ \mathrm{for}\ d = 1, ..., p,\]
\[Y=\sin(\theta X)+\kappa \epsilon.\]

\item \texttt{Sine\ Period\ 16$\pi$}$\left( X, Y \right) \in \Real^p \times \Real^p$: Same as above except $\theta = 16 \pi$ and the noise on $Y$ is changed to $0.5 \kappa \epsilon$.

\item \texttt{Square}$\left( X, Y \right) \in \Real^p \times \Real^p$: For $U \sim \mathcal{U} \left( -1, 1 \right)$, $V \sim \mathcal{U} \left( -1, 1 \right)$, $\epsilon \sim {\mathcal{N} \left( 0, 1 \right)}^p$, $\theta = -\frac{\pi}{8}$,
\[X_{\left| d \right|} = U \cos \left( \theta \right) + V \sin \left( \theta \right) + 0.05 p \epsilon_{\left| d \right|},\]
\[Y_{\left| d \right|} = -U \sin \left( \theta \right) + V \cos \left( \theta \right).\]

\item \texttt{Diamond}$\left( X, Y \right) \in \Real^p \times \Real^p$: Same as above except $\theta = \pi/4$.

\item \texttt{Two\ Parabolas}$\left( X, Y \right) \in \Real^p \times \Real$: For $\epsilon \sim \mathcal{U} \left( 0, 1 \right)$, $U \sim \mathcal{B} \left( 0.5 \right)$,
\[X \sim {\mathcal{U} \left( -1, 1 \right)}^p,\]
\[Y = \left( {\left( w \T X \right)}^2 + 2 \kappa \epsilon \right) \cdot \left(U - \frac{1}{2} \right).\]

\item \texttt{Circle}$\left( X, Y \right) \in \Real^p \times \Real$: For $U \sim {\mathcal{U} \left( -1, 1 \right)}^p$, $\epsilon \sim \mathcal{N} \left( 0, I_p \right)$, $r = 1$,
\[X_{\left| d \right|} = r \left( \sin \left( \pi U_{\left| d + 1 \right|} \right) \prod \limits_{j = 1}^d \cos \left( \pi U_{\left| j \right|} \right) + 0.4 \epsilon_{\left| d \right|} \right)\ \mathrm{for}\ d = 1, ..., p-1,\]
\[X_{\left| d \right|} = r \left( \prod \limits_{j = 1}^p \cos \left(\pi U_{\left| j \right|} \right) + 0.4 \epsilon_{\left| p \right|} \right),\]
\[Y_{\left| d \right|} = \sin \left(\pi U_{\left| 1 \right|} \right).\]

\item \texttt{Ellipse}$\left( X, Y \right) \in \Real^p \times \Real^p$: Same as above except $r = 5$.

\item \texttt{Multiplicative\ Noise}$\left( x, y \right) \in \Real^p \times \Real^p$: $u \sim \mathcal{N} \left( 0, I_p \right)$,
\[x \sim \mathcal{N} \left( 0, I_p \right),\]
\[y_{\left| d \right|} = u_{\left| d \right|} x_{\left| d \right|}\ \mathrm{for}\ d = 1, ..., p.\]

\item \texttt{Multimodal\ Independence}$\left( X, Y \right) \in \Real^p \times \Real$: For $U \sim \mathcal{N} \left( 0, I_p \right)$, $V \sim \mathcal{N} \left( 0, I_p \right)$, $U' \sim {\mathcal{B} \left( 0.5 \right)}^p$, $V' \sim {\mathcal{B} \left( 0.5 \right)}^p$,
\[X = U/3 + 2U' - 1,\]
\[Y = V/3 + 2V' - 1.\]
\end{enumerate}
